# Supplementary material for: ForceVLA2: Unleashing Hybrid Force-Position Control with Force Awareness for Contact-Rich Manipulation
Source: arXiv:2603.15169 source file (2026-03-16)
Supplement: Supplementary file 1 [file supp.tex]

% CVPR 2026 Paper Template; see https://github.com/cvpr-org/author-kit

\documentclass[10pt,twocolumn,letterpaper]{article}

%%%%%%%%% PAPER TYPE  - PLEASE UPDATE FOR FINAL VERSION
% \usepackage{cvpr}              % To produce the CAMERA-READY version
\usepackage[review]{tips/cvpr}      % To produce the REVIEW version
% \usepackage[pagenumbers]{cvpr} % To force page numbers, e.g. for an arXiv version

% Import additional packages in the preamble file, before hyperref
%% This file contains a number of tweaks that are typically applied to the main document.
%% They are not enabled by default, but can be enabled by uncommenting the relevant lines.

%%
%% Inline annotations; for predefined colors, refer to "dvipsnames" in the xcolor package:
%% https://tinyurl.com/overleaf-colors
%%

%%
%% disable for camera ready / submission by uncommenting these lines  
%%
% \renewcommand{\TODO}[1]{}
% \renewcommand{\todo}[1]{#1}

%%
%% work harder in optimizing text layout. Typically shrinks text by 1/6 of page, enable
%% it at the very end of the writing process, when you are just above the page limit
%%
% \usepackage{microtype}

%%
%% fine-tune paragraph spacing
%%
% \renewcommand{\paragraph}[1]{\vspace{.5em}\noindent\textbf{#1.}}

%%
%% globally adjusts space between figure and caption
%%
% \setlength{\abovecaptionskip}{.5em}

%%
%% Allows "the use of \paper to refer to the project name"
%% with automatic management of space at the end of the word
%%
% \usepackage{xspace}
% \newcommand{\paper}{ProjectName\xspace}

%%
%% Commonly used math definitions
%%
% \DeclareMathOperator*{\argmin}{arg\,min}
% \DeclareMathOperator*{\argmax}{arg\,max}

%%
%% Tigthen underline
%%
% \usepackage{soul}
% \setuldepth{foobar}
\usepackage{lipsum}  % plase holder

% It is strongly recommended to use hyperref, especially for the review version.
% hyperref with option pagebackref eases the reviewers' job.
% Please disable hyperref *only* if you encounter grave issues, 
% e.g. with the file validation for the camera-ready version.
%
% If you comment hyperref and then uncomment it, you should delete *.aux before re-running LaTeX.
% (Or just hit 'q' on the first LaTeX run, let it finish, and you should be clear).
\definecolor{cvprblue}{rgb}{0.21,0.49,0.74}
\usepackage[pagebackref,breaklinks,colorlinks,allcolors=cvprblue]{hyperref}
%%%%%%%%%zhqadd%%%%%%%%%%%%%%%
\usepackage{color}
\usepackage{tabularray}
\usepackage{bbding}
\UseTblrLibrary{diagbox}
%%%%%%%%%zhqadd%%%%%%%%%%%%%%%

%%%%%%%%% PAPER ID  - PLEASE UPDATE
% \def\paperID{10859} % *** Enter the Paper ID here

%%%%%%%%% TITLE - PLEASE UPDATE
% \title{
% Foca-VLA:
% Unleashing Hybrid Force-Position Control with Force Awareness \\
% for Contact-Rich Manipulation
% \\ }

\title{Foca-VLA:
Unleashing Hybrid Force-Position Control with Force Awareness \\ 
for Contact-Rich Manipulation\\
\textit{Supplementary Materials} }
% for Enhanced VLA in Contact-Rich Manipulation}
% HopMan: Hybrid Force-Position Control for Delicate Manipulation} 
% \\in Embodied Intelligence Systems}
%Embodied Impedance Controlling for Robot Precise Manipulaitons Based on VLA MoE

%%%%%%%%% AUTHORS - PLEASE UPDATE
\author{First Author\\
Institution1\\
Institution1 address\\
{\tt\small firstauthor@i1.org}
% For a paper whose authors are all at the same institution,
% omit the following lines up until the closing ``}''.
% Additional authors and addresses can be added with ``\and'',
% just like the second author.
% To save space, use either the email address or home page, not both
\and
Second Author\\
Institution2\\
First line of institution2 address\\
{\tt\small secondauthor@i2.org}
}

\usepackage[pagebackref,breaklinks,colorlinks]{hyperref}
\usepackage{color}
\usepackage{caption, subcaption, multirow, overpic, textpos}
\usepackage{bbm}
\usepackage{titletoc}
\usepackage{graphicx}

\usepackage{colortbl}
\usepackage{tcolorbox}

% for tables
\usepackage{multirow}
\usepackage{booktabs}
\usepackage{makecell}

% For theorems and such
\usepackage{amsmath}
\usepackage{amssymb}
\usepackage{mathtools}
\usepackage{amsthm}

% if you use cleveref..
\usepackage[capitalize,noabbrev]{cleveref}

\definecolor{iccvblue}{RGB}{0, 102, 204}
\hypersetup{
    colorlinks=true, 
    citecolor=iccvblue,
}

%%%%%%%%%%%%%%%%%%%%%%%%%%%%%%%%
% THEOREMS
%%%%%%%%%%%%%%%%%%%%%%%%%%%%%%%%

\usepackage{bm}
\usepackage{tocbasic}

%
% --- inline annotations
%
% \usepackage[dvipsnames]{xcolor}
% \newcommand{\red}[1]{{\color{red}#1}}
% \newcommand{\todo}[1]{{\color{red}#1}}
% \newcommand{\TODO}[1]{\textbf{\color{red}[TODO: #1]}}

% Support for easy cross-referencing
% \usepackage[pagebackref,breaklinks,colorlinks]{hyperref}
\crefname{section}{Sec.}{Secs.}
\Crefname{section}{Section}{Sections}
\Crefname{table}{Table}{Tables}
\crefname{table}{Tab.}{Tabs.}
\crefname{figure}{Fig.}{Figs.}
\crefname{equation}{Eq.}{Eqs.}

\definecolor{Gray}{gray}{0.9}
\definecolor{LightCobaltBlue}{RGB}{143,170,220}
\definecolor{Amber}{RGB}{255,102,0}
\definecolor{BlackOlive}{RGB}{59,56,56}
\definecolor{AlloyOrange}{RGB}{197,90,17}
\definecolor{B'dazzledBlue}{RGB}{47,85,151}
\definecolor{DarkBlue}{RGB}{72, 116, 203}
\definecolor{DarkGreen}{RGB}{106, 169, 63}

\definecolor{baselinecolor}{gray}{.9}

\definecolor{deemph}{gray}{0.6}

% \newcommand{\baseline}[1]{\cellcolor{baselinecolor}{#1}}
% New light cyan color
\definecolor{lightcyan}{RGB}{230,250,250} % or tweak to {230,250,250} for softer tone

% \newcommand{\authorskip}{\hspace{2.5mm}}

% \definecolor{baselinecolor}{lightcyan}{.9}

\begin{document}
% \maketitle

\twocolumn[{%
\renewcommand\twocolumn[1][]{#1}%
\maketitle
}]
\input{sec/X_suppl}

% WARNING: do not forget to delete the supplementary pages from your submission 
% \input{sec/X_suppl}

\end{document}
